# Supplementary material for: Learning to Localize, Grasp, and Hand Over Unmodified Surgical Needles
Source: arXiv:2112.04071 source file (2021-12-08)
Supplement: Supplementary file 1 [file 9-appendix.tex]

\section*{Appendix} \label{sec:appendix}

My appendix was removed
